# Supplementary material for: MIRA: Mental Imagery for Robotic Affordances
Source: arXiv:2212.06088 source file (2022-12-12)
Supplement: Supplementary file 1 [file supp.tex]

\documentclass{article}
\usepackage[usenames,dvipsnames]{xcolor}

% Added by Yen-Chen
\include{macros}
\include{listings}
\usepackage{amssymb}
\usepackage{graphicx}
\usepackage{subcaption}
\usepackage[inline]{enumitem}
\usepackage{booktabs} % for professional tables
\usepackage{colortbl}
\usepackage{wrapfig}
\usepackage[subtle]{savetrees}
\usepackage{pifont}% http://ctan.org/pkg/pifont
\usepackage[most]{tcolorbox}
\usepackage[font=small,labelfont=bf,tableposition=top]{caption}
\newcolumntype{x}[1]{>{\centering\arraybackslash\hspace{0pt}}p{#1}}
\usepackage{xspace}

\usepackage{corl_2022} % Use this for the initial submission.
%\usepackage[final]{corl_2022} % Uncomment for the camera-ready ``final'' version.
%\usepackage[preprint]{corl_2022} % Uncomment for pre-prints (e.g., arxiv); This is like ``final'', but will remove the CORL footnote.

%\title{NoVA: Novel View Affordance Synthesis \\for Robotic Manipulation}
\title{MIRA: Mental Imagery for Robotic Affordances\\Supplementary Material}

% The \author macro works with any number of authors. There are two
% commands used to separate the names and addresses of multiple
% authors: \And and \AND.
%
% Using \And between authors leaves it to LaTeX to determine where to
% break the lines. Using \AND forces a line break at that point. So,
% if LaTeX puts 3 of 4 authors names on the first line, and the last
% on the second line, try using \AND instead of \And before the third
% author name.

% NOTE: authors will be visible only in the camera-ready and preprint versions (i.e., when using the option 'final' or 'preprint'). 
% 	For the initial submission the authors will be anonymized.

\author{
  Jane E.~Doe\\
  Department of Electrical Engineering and Computer Sciences\\
  University of California Berkeley 
  United States\\
  \texttt{janedoe@berkeley.edu} \\
  %% examples of more authors
  %% \And
  %% Coauthor \\
  %% Affiliation \\
  %% Address \\
  %% \texttt{email} \\
  %% \AND
  %% Coauthor \\
  %% Affiliation \\
  %% Address \\
  %% \texttt{email} \\
  %% \And
  %% Coauthor \\
  %% Affiliation \\
  %% Address \\
  %% \texttt{email} \\
  %% \And
  %% Coauthor \\
  %% Affiliation \\
  %% Address \\
  %% \texttt{email} \\
}

\begin{document}
\maketitle
%===============================================================================
\appendix
\section{CUDA Kernel for Orthographic Ray Casting}
\begin{lstlisting}[language=C++, label=code:orthographic, caption=CUDA kernel for orthographic ray casting in instant-NGP~\cite{mueller2022instant}.]

inline __host__ __device__ Ray pixel_to_ray_orthographic(
	uint32_t spp,
	const Eigen::Vector2i& pixel,
	const Eigen::Vector2i& resolution,
	const Eigen::Vector2f& focal_length,
	const Eigen::Matrix<float, 3, 4>& camera_matrix,
	const Eigen::Vector2f& screen_center,
	float focus_z = 1.0f,
	float dof = 0.0f
) {
	auto uv = pixel.cast<float>().cwiseQuotient(resolution.cast<float>());

	Eigen::Vector3f dir = {
		0.0f,
		0.0f,
		1.0f
	};
	dir = camera_matrix.block<3, 3>(0, 0) * dir;

	Eigen::Vector3f offset_x = {
		(uv.x() - screen_center.x()) * (float)resolution.x() / focal_length.x(),
		0.0f,
		0.0f
	};
	offset_x = camera_matrix.block<3, 3>(0, 0) * offset_x;
	Eigen::Vector3f offset_y = {
		0.0f,
		(uv.y() - screen_center.y()) * (float)resolution.y() / focal_length.y(),
		0.0f
	};
	offset_y = camera_matrix.block<3, 3>(0, 0) * offset_y;

	Eigen::Vector3f origin = camera_matrix.col(3);
	origin = origin + offset_x + offset_y;

	return {origin, dir};
\end{lstlisting}
\bibliography{example}  % .bib
\end{document}
